# Supplementary material for: Instance-Aware Predictive Navigation in Multi-Agent Environments
Source: arXiv:2101.05893 source file (2021-01-14)
Supplement: Supplementary file 1 [file appendix.tex]

\section{More Details about Experiments}
We introduce more details about experiments in this section.

\minisection{map configuration} we conduct experiments on two maps in CARLA, \texttt{town01} and \texttt{town02}. One key setting is where the ego-vehicle is spawned at the beginning of simulator booting. To fully explore the environments, we selected spawning points on the two maps to cover different regions and made the ego-vehicle spawned randomly on these spawning points. The map configuration and spawning points are visualized in Fig. \ref{fig:map}.

\begin{figure}[htbp]
\centering
\subfigure[]{
    \begin{minipage}{.35\linewidth}
        \centering
        \includegraphics[height=8\baselineskip]{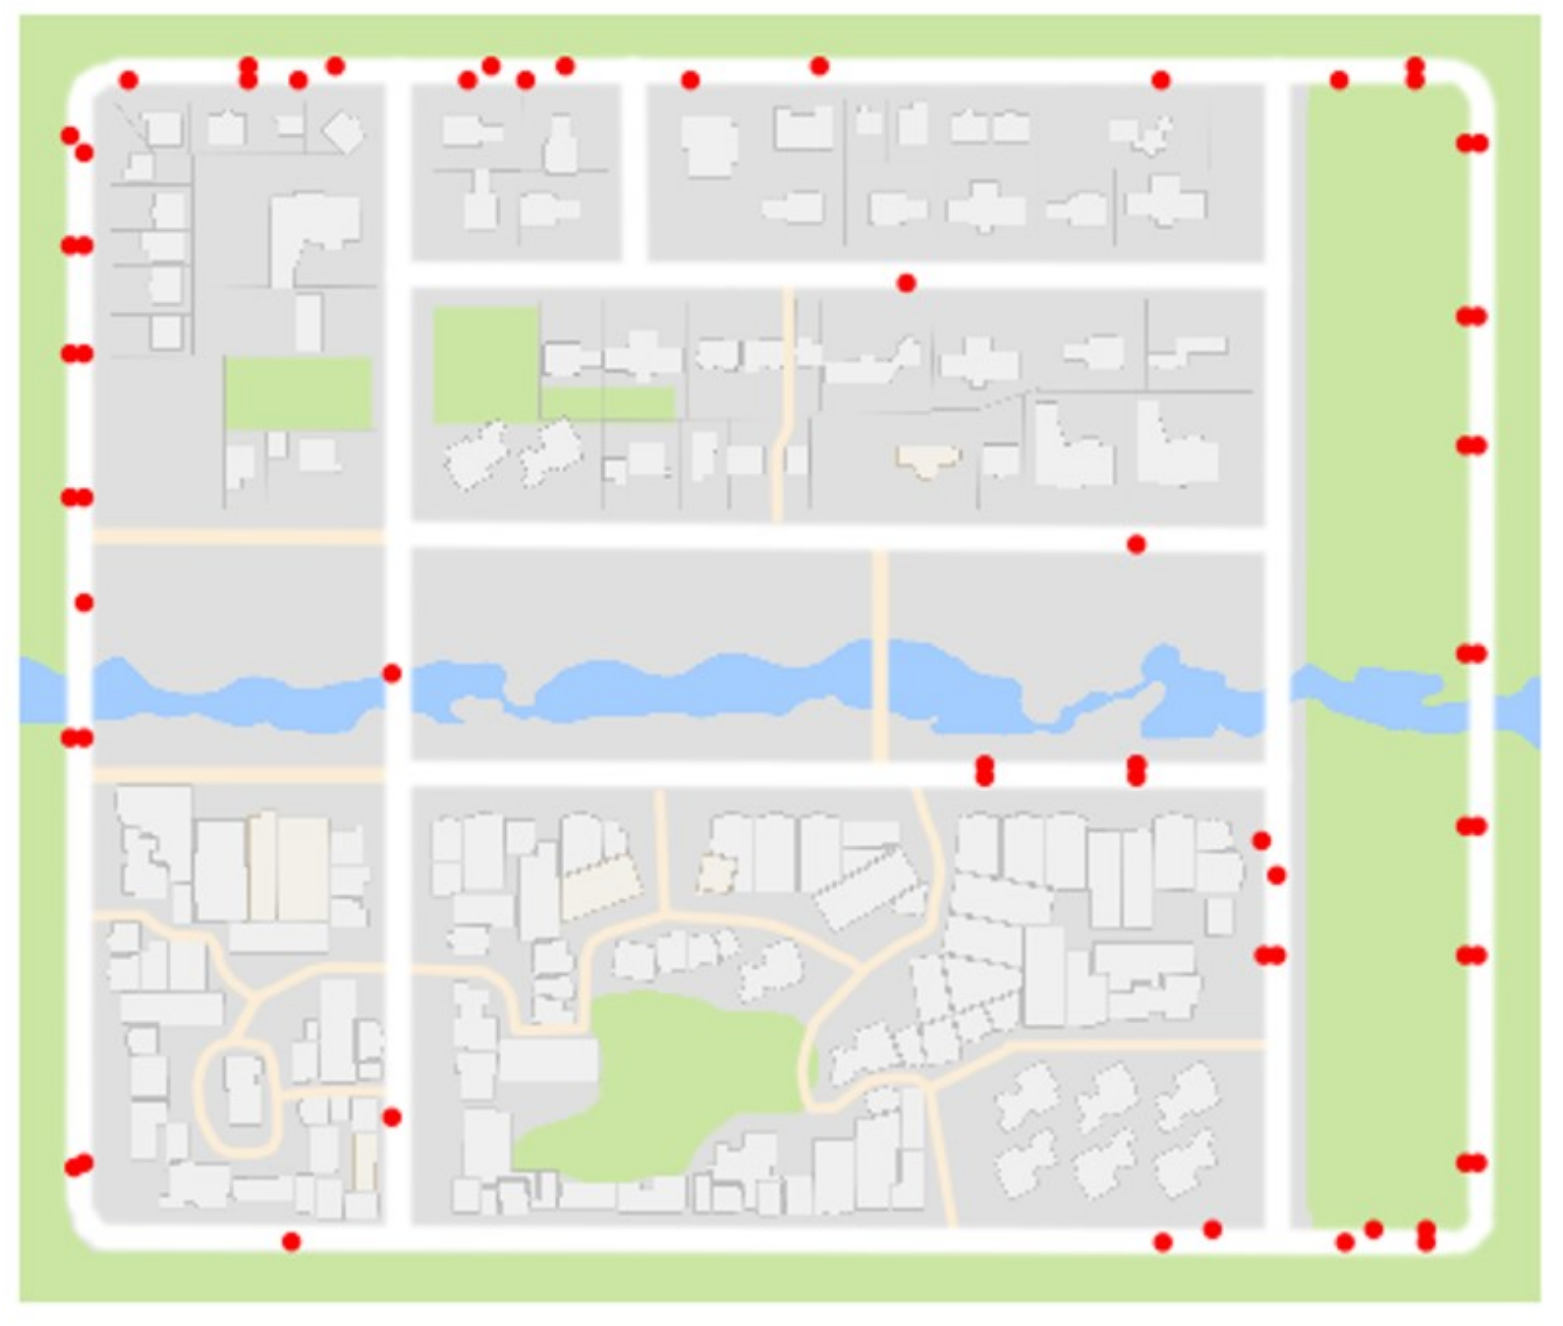}
    \end{minipage}
}
\qquad
\subfigure[]{
    \begin{minipage}{.35\linewidth}
        \centering
        \includegraphics[height=8\baselineskip]{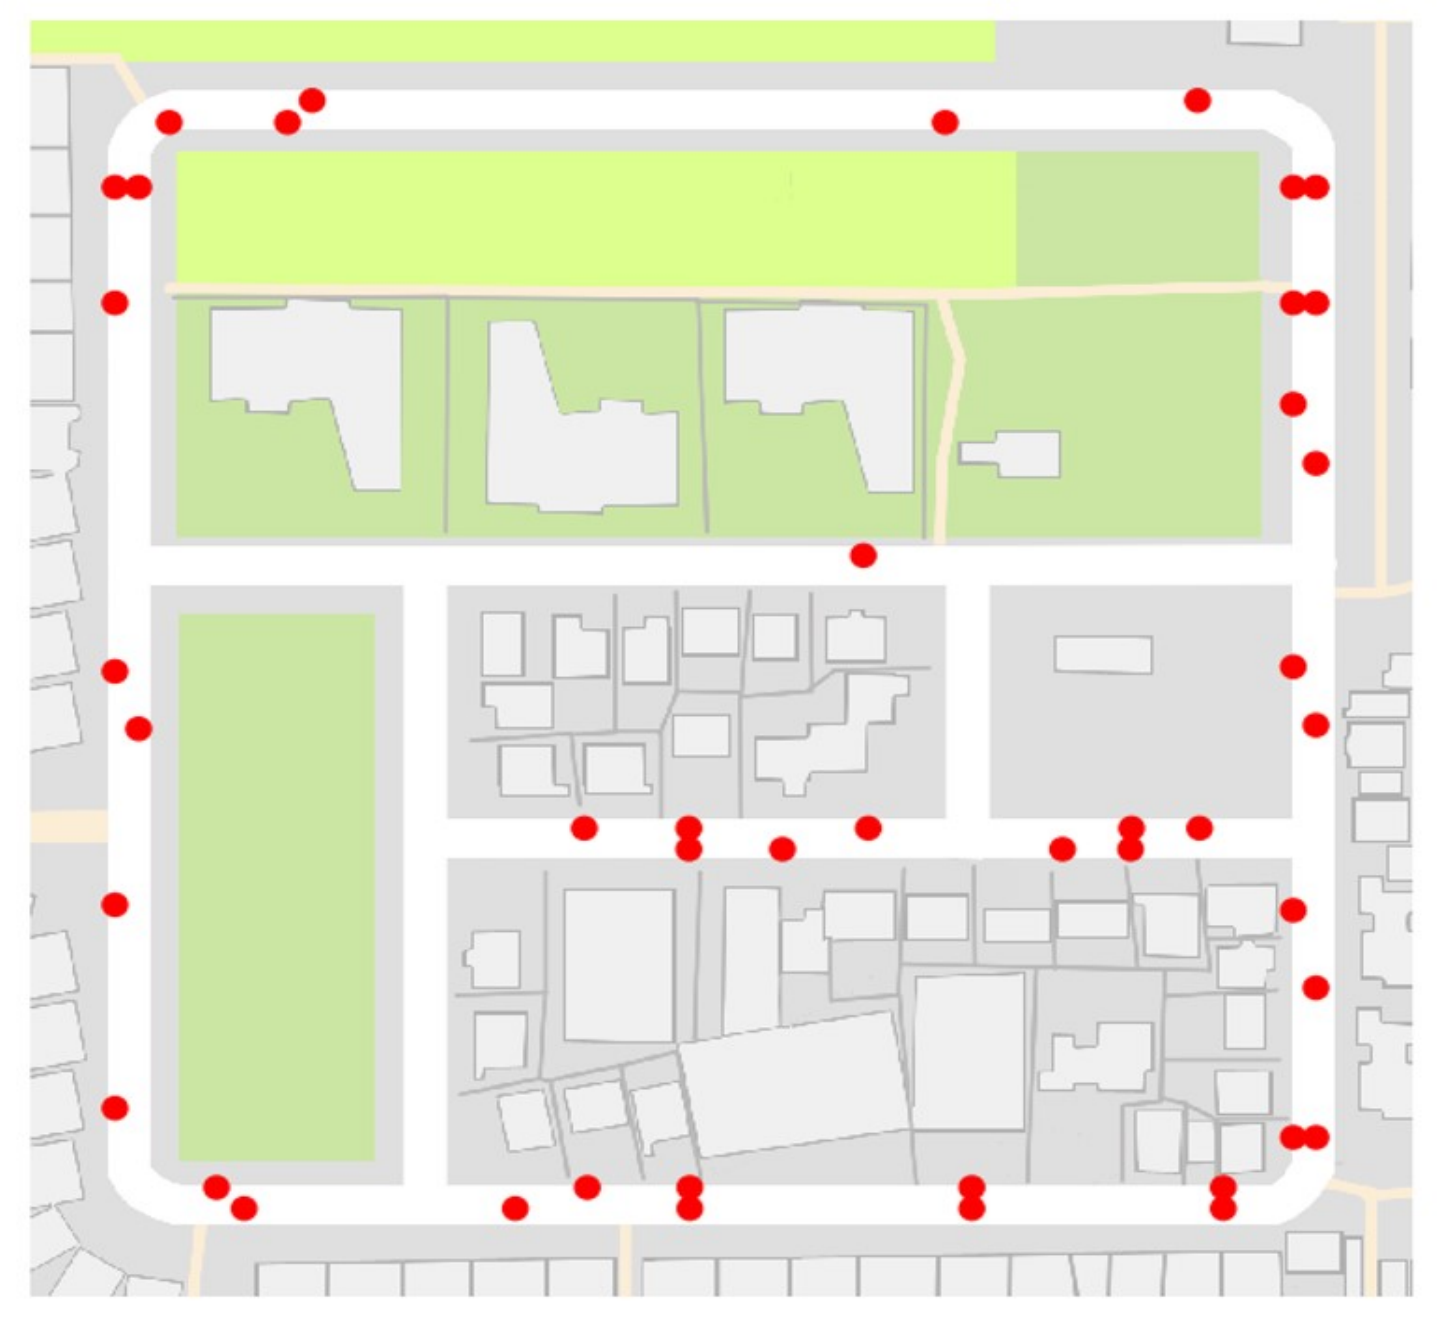}
    \end{minipage}
}
\caption{The map configuration and ego-vehicle spawning points in CARLA (a) \texttt{town01}, (b) \texttt{town02}.}
\label{fig:map}
\end{figure}

\minisection{model pretraining on CARLA} when training on CARLA, one issue is the absence of other agents in the observation of some frames. We found this influence the model training a lot, especially when this happens frequently at the beginning of model training. So to have the model training start more smoothly, we collected a dataset from CARLA simulator including the full information used in \model.
